# Supplementary material for: Lecture Notes on Quantum Algorithms for Scientific Computation
Source: arXiv:2201.08309 source file (2022-01-20)
Supplement: Supplementary file 1 [file appendix.tex]

\appendix
\chapter{Notation}

We use the following asymptotic notations besides the usual $\Or$ (or ``big-O'') notation: 
we write $f=\Omega(g)$ if $g=\Or(f)$; $f=\Theta(g)$ if $f=\Or(g)$ and $g=\Or(f)$; $f=\wt{\Or}(g)$ if $f=\Or(g\operatorname{polylog}(g))$.

We use $\|\cdot\|$ to denote vector or matrix 2-norm: when $v$ is a vector we denote by $\|v\|$ its 2-norm, and when $A$ is matrix we denote by $\|A\|$ its operator norm. For two quantum states $\ket{x}$ and $\ket{y}$, we sometimes write $\ket{x,y}$ to denote $\ket{x}\ket{y}$. We use fidelity to measure how close to each other two quantum states are. Note there are two common definitions for the fidelity between two pure states $\ket{\phi}$ and $\ket{\varphi}$: it is either $|\braket{\phi|\varphi}|$ or $|\braket{\phi|\varphi}|^2$. 

Unless otherwise specified, a vector $v\in\CC^N$ is an unnormalized vector, and a normalized vector (stored as a quantum state) is denoted by $\ket{v}=v/\norm{v}$.
A vector $v$ can be expressed in terms of $j$-th component as $v=(v_j)$ or $(v)_j=v_j$. We use a $0$-based indexing, i.e. $j=0,\ldots,N-1$ or $j\in [N]$. When $1$-based indexing is used, we will explicitly write $j=1,\ldots,N$.

\chapter{Basic computational complexity theory}
